# Supplementary material for: Degeneracy-breaking and Long-lived Multimode Microwave Electromechanical Systems Enabled by Cubic Silicon-Carbide Membrane Crystals
Source: arXiv:2401.01020 ancillary file (2025-02-11)
Supplement: Supplementary file 1 [file supplementary-information.pdf]

# Supplementary Information for “Long-lived Microwave Electromechanical Systems Enabled by Cubic Silicon-Carbide Membrane Crystals”

Yulong Liu,<sup>1,2,\*</sup> Huanying Sun,<sup>1</sup> Qichun Liu,<sup>1</sup> Haihua Wu,<sup>1</sup> Mika A. Sillanpää,<sup>2</sup> and Tiefu Li<sup>3,†</sup>

<sup>1</sup>*Beijing Academy of Quantum Information Sciences, Beijing 100193, China*

<sup>2</sup>*Department of Applied Physics, Aalto University, P.O. Box 15100, FI-00076 Aalto, Finland*

<sup>3</sup>*School of Integrated Circuits and Frontier Science Center for Quantum Information, Tsinghua University, Beijing 100084, China*  
(Dated: January 2, 2024)

This Supplementary Information includes:

- Supplementary Notes 1-3
- Supplementary Figures 1-4
- Supplementary Tables 1

---

\* liuyul@baqis.ac.cn

† litf@tsinghua.edu.cn

This Supplementary Information is organized as follows: In Supplementary Note 1, we describe the fabrication process of 3C-SiC microwave cavity electromechanical device studied in this work. In Supplementary Note 2, we present the microwave measurement setups. The calibration of initial thermal occupation of the mechanical mode and its PSD curves as increasing the sideband pump power are presented in Supplementary Note 3. Devices parameters are summarized in Supplementary Tables 1.

### SUPPLEMENTARY NOTE 1. THE DEVICE STRUCTURE AND ITS FABRICATION PROCESSES

Long-lived phonons have gained significant interest in the field of quantum technology due to their potential applications in various areas such as excellent carriers of quantum information, high-precision sensing, and efficient transducers between different types of quantum systems, et al. Here in this work, we will explore long-lived mechanical modes in 3C-SiC membrane and construct coherent electromechanical interface between microwave photons and long-lived phonons.

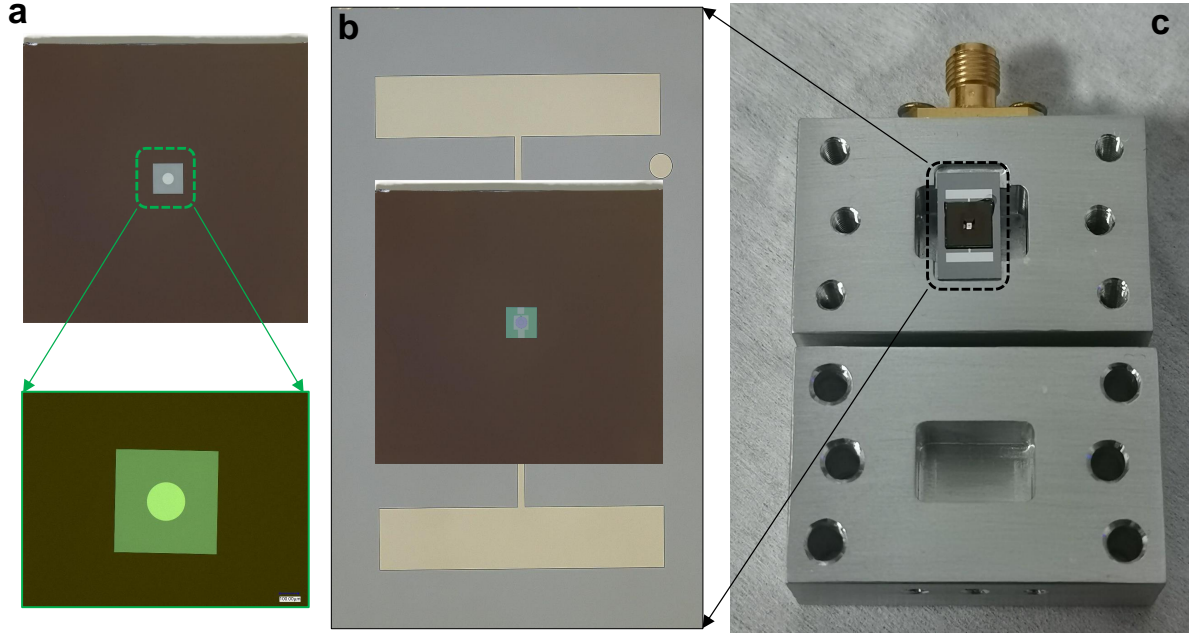

Supplementary Figure 1. **a** The metalized 3C-SiC membrane chip. Inset is the zoomed-in view of the membrane window with circular Al pad. **b** Mechanical capacitor chip consists of bottom microwave antenna electrode and upper membrane mechanical resonator. **c** 3D microwave cavity electromechanical interface with embedded 3C-SiC mechanical capacitor. The SMA connector is used to coupling the microwave signals in and out from 3D superconducting microwave resonator.

The 3C-SiC membrane chip is shown in Supplementary Figure 1a. The silicon frame is in a size of  $5\text{ mm} \times 5\text{ mm}$ , and the thickness is  $400\text{ }\mu\text{m}$ . A layer of cubic crystalline SiC with a thickness of  $50\text{ nm}$  was grown epitaxially on both sides of the silicon substrate. Wet etching with potassium hydroxide, an SiC window is opened and the suspend SiC membrane is in a size of  $500\text{ }\mu\text{m} \times 500\text{ }\mu\text{m}$ . We started with a  $20\text{ nm}$  aluminum film evaporated (JEB-4, Adnanotek) on the entire front side of the 3C-SiC chip. The evaporation rate is  $0.2\text{ nm/s}$  with a substrate spin speed at  $10\text{ rpm}$ . Negative tone photoresist (ma-N 2410) was spincoated onto the front side again after evaporation. The spinning rate was  $4000\text{ rpm}$  and operating for  $1\text{ minute}$ . The chip with resist was then baked at  $90\text{ }^\circ\text{C}$  for  $3\text{ minutes}$ . The pattern of a  $200\text{ }\mu\text{m}$ -radius circle was transferred onto the membrane via electron beam lithography (Sigma 300, Zeiss) using a dose around  $169\text{ }\mu\text{C/cm}^2$ . The development process was continued in the ma-D525 developer for around  $15\text{ minutes}$  at room temperature. The zoomed-in subfigure of Supplementary Figure 1a shows an optical image of the metalized 3C-SiC membrane window.

Using flip-chip bonder (ACC $\mu$ RA), we ensemble the mechanical capacitor by flipping and aligning the center of electrodes on the upper and lower chips. The size of bottom microwave-antenna chip is  $6.5\text{ mm} \times 10.5\text{ mm}$ . The bottom antenna electrode is obtained by further processing a silicon substrate by sputtering a thin layer of  $120\text{ nm}$  niobium. Unnecessary metal films other than the electrode pattern are etched away by reactive ion etching (RIE). The detailed etching recipe is shown in Supplementary Table 1. The mechanical capacitor chip is shown in Supplementary Figure 1b. This forms the structure of parallel-plate capacitor with a narrow vacuum gap. The mechanical capacitor chip is then embedded in the geometric center of the 3D microwave cavity

where the maximum electric field locates in. The radiation pressure of microwave photon can move the metalized SiC membrane with a displacement of  $\hat{x}$ , introducing an adjustable mechanical capacitance  $C_m(\hat{x})$  to the 3D microwave cavity. The mechanical vibration in turn changes the cavity resonance frequency, forming dispersive type cavity optomechanical interaction.

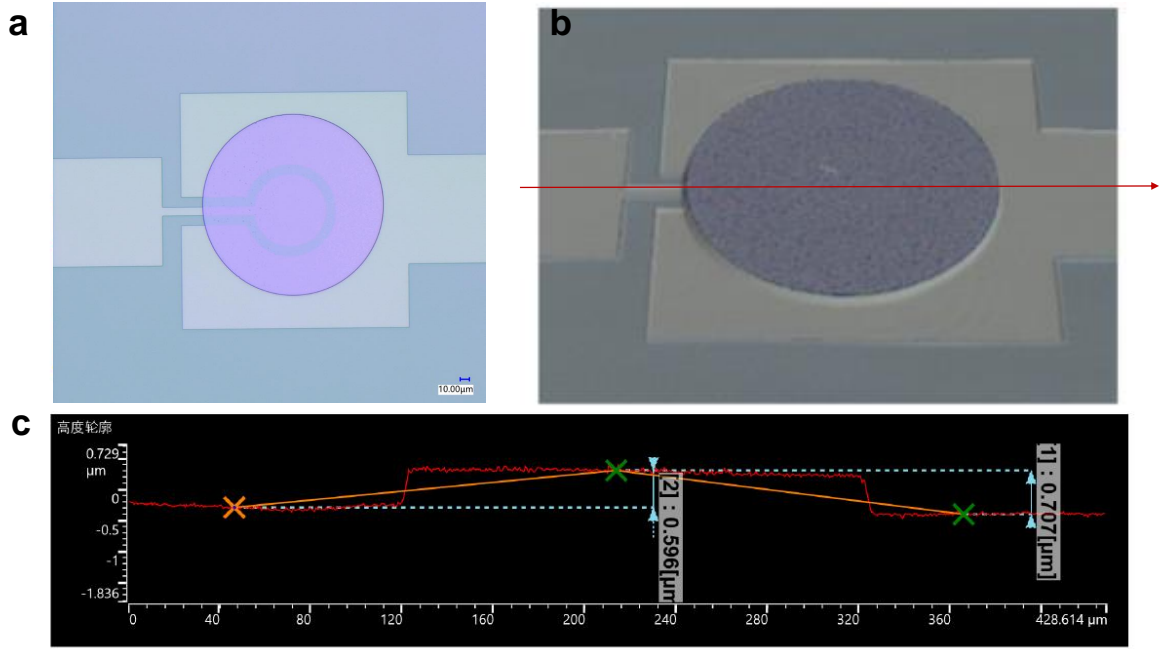

Supplementary Figure 2. **a** The pattern of the upper and bottom electrodes of mechanical capacitor. **b** 3D laser microscope pattern of the parallel-plate area. **c** The amplitude profile corresponding to the red-solid line-cut in **b**.

The optomechanical coupling strength is one of the key parameter for the explore device applications in both the fundamental research and quantum technologies. The optical microscope pattern of the upper and bottom electrodes of mechanical capacitor is shown in Supplementary Figure 2a. The vacuum optomechanical coupling strength  $g_0$  is mainly determined by the gap of mechanical capacitors. We use the 3D laser microscope to get the surface topography and then infer the value of this gap. Supplementary Figure 2b shows the outline map (using LEXT) of the parallel-plate area. The height profile (corresponding to the red-solid line-cut area of Supplementary Figure 2b) is shown in Supplementary Figure 2c, from which we infer the vacuum gap is around 576 nm.

Supplementary Table 1. The RIE etching parameters used in system RIE-10NR (Samco Inc.).

| Procedure | Gas             | Pressure (Pa) | Flow rate (sccm) | Power (W) | Time (s) |
|-----------|-----------------|---------------|------------------|-----------|----------|
| 1         | O <sub>2</sub>  | 5             | 50               | 50        | 20       |
| 2         | CF <sub>4</sub> | 2             | 30               | 100       | 100      |

## SUPPLEMENTARY NOTE 2. MEASUREMENT SETUPS AND METHODS

The device is mounted on the 10 mK mixing-chamber layer of a dilution refrigerator. The detailed measurement schematic diagram is shown in Supplementary Figure 3. An arbitrary waveform generator (Tektronix AWG5014C) with IQ-mixers are used to shape the pump-tones (marked by red-color is with a frequency of  $\omega_c - \omega_m$ ), amplify-tone (marked by blue colors is with a frequency of  $\omega_c + \omega_m$ ), and the signal-tone (marked by green color is with a frequency of  $\omega_c$ ) to pulses in the time domain. These three tones are combined at room temperature with splitters, and then transmitted down through the input line until they pass through an SMA coupler and into the interior of the 3D microwave cavity. Since the device has only one SMA coupling port, here we use a circulator to isolate the input and output signals of the 3D cavity electromechanical device. To increase the on-off ratio of the pulse, we have used a high speed microwave switcher following the mixer for each tone, respectively. While the AWG analog channel outputs a pulse waveform signal to the mixer, the maker channel generates a control signal for fast

switching. Immediately following the output port of the circulator, the canceling line is coupled to the microwave output line through a directional coupler. By adjusting the amplitude and phase of canceling tone, the reflected pump-tone (amplify-tone) can be canceled effectively to avoid the saturation of HEMT. A real-time signal analyzer (Tektronix RSA5126B) is used for digital sampling and analysing the output signal. All instruments are phase-locked by a 10 MHz rubidium frequency standard. For the signal pulse measurement, the RSA acquiring frequency center is a bit shifted from signal-tone (fixed at  $\omega_c/2\pi - 400$  Hz), to make the acquired IQ signal having a small oscillation frequency. The delay time from write-in to read-out is controlled by the AWG in time domain. To synchronize the RSA signal acquisition with signal pulse, the RSA is triggered by an AWG pulse. Under the pulse sequence, We can measure both the quadratures of motion encoded in a recovered optomechanical sideband signals. Repeating this pulse sequence allows us to capture the quadrature distribution of the recovered microwave states, realizing the quantum tomography. It is notable that, the exponential rising rate of the encoded pulse signal are optimised to be the optical-damping rate of mechanical mode to obtain the maximum signal capture efficiency. In addition to the state tomography, when taking the  $S$  parameter measurement and spectrum measurement, the PNA (Agilent N5232A) probe tone is combined into the input line. Meanwhile, the amplify-tone and signal-tone are keeping off, and the pump-tone is always keeping on by the AWG.

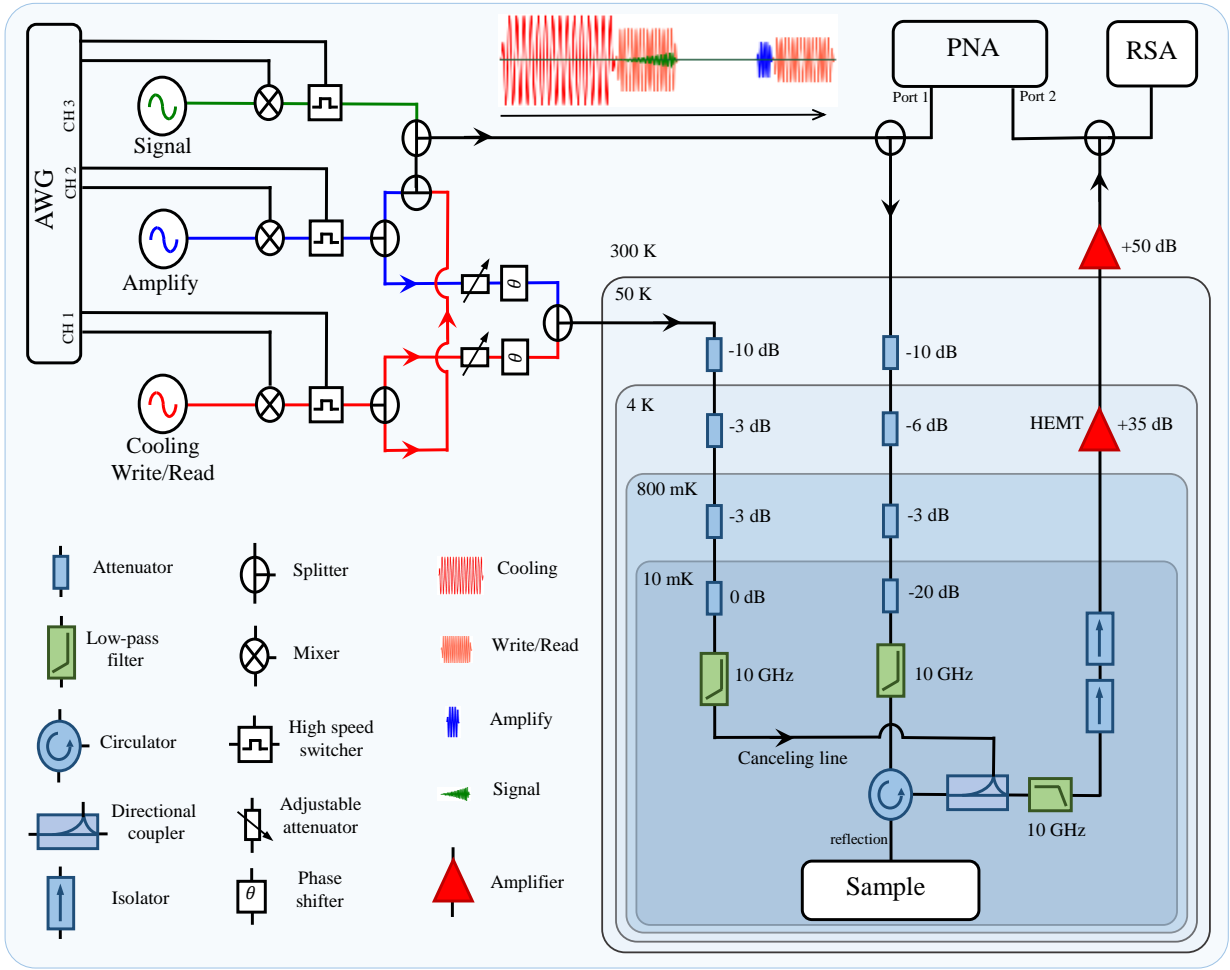

Supplementary Figure 3. The detailed experimental measurement schematic diagram. A cryogenic circulator is used to separate the incident and reflected signals, defining the input and output ports of the 3D microwave cavity electromechanical device. The pulse-sequence and measurement setups are described in detail here. Microwave generators creates the sideband cooling tone (also plays the role of writing and readout of the microwave pulse-signal) with a frequency red-detuned to the cavity resonance. The cooling (writing and reading) tones are marked by red-color in the measurement schematic diagram. The second arm is used to cancel the cooling tone before HEMT amplification, in order to avoid saturating the low-noise amplifier with the microwave cooling tone. Using optomechanical amplification technique with a blue-sideband pump, we intrinsically amplify the mechanical motion with a gain around 48 dB with a minimal added noise. The signal tone is encode in a pulse with the shape of exponential rising with a rate of  $\gamma_{\text{opt}}^g$ .

### SUPPLEMENTARY NOTE 3. TEMPERATURE SWEEP AND THE SIDEBAND COOLING PSD SPECTRA

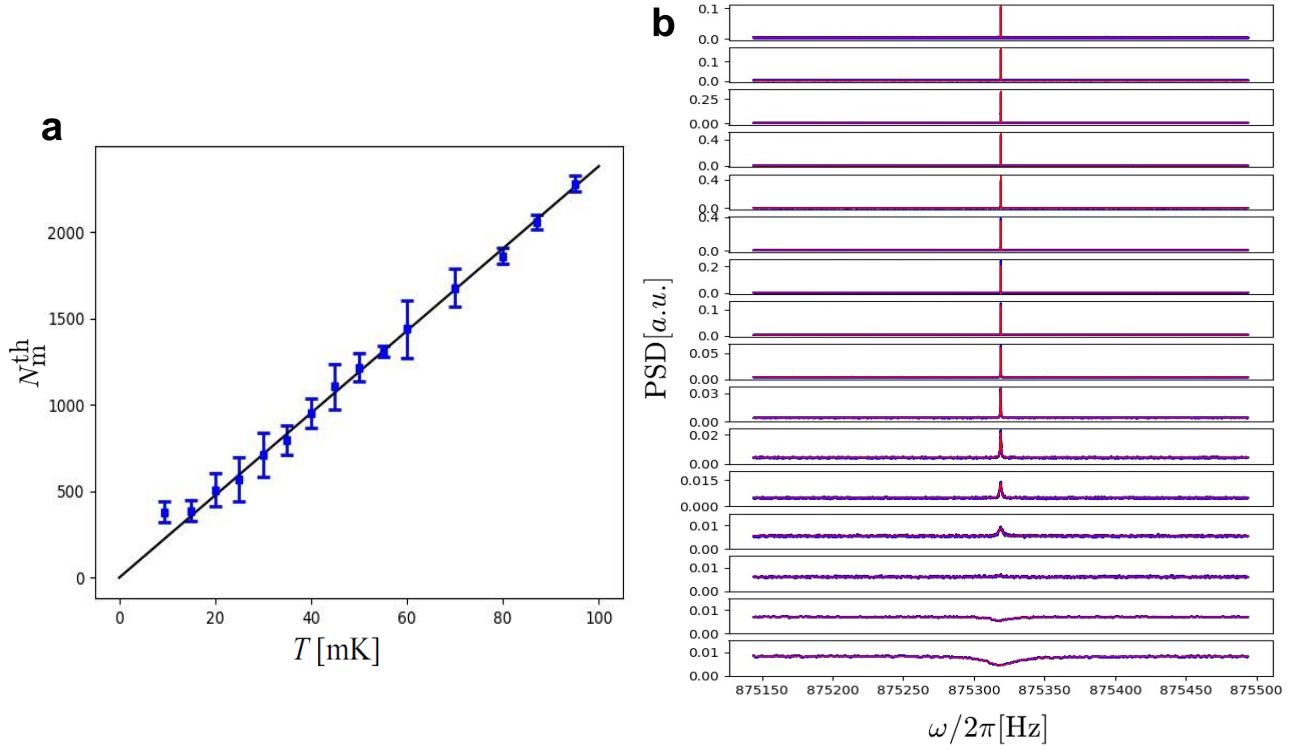

Supplementary Figure 4. **a** The metalized 3C-SiC membrane chip. Inset is the zoomed-in view of the membrane window with circular Al pad. **b** Mechanical capacitor chip consists of bottom microwave antenna electrode and upper membrane mechanical resonator. **c** 3D microwave cavity electromechanical interface with embedded 3C-SiC mechanical capacitor. The SMA connector is used to coupling the microwave signals in and out from 3D superconducting microwave resonator.

In this section, we will show the calibration of initial mode temperature and thermal phonon occupation of the 3C-SiC drumhead mechanical mode. We measure the PSD of the output microwave field as increasing the cryostat operating temperature from 8.5 mK to 100 mK. The thermal phonon occupation are presented in Supplementary Figure 4a, where we found that the mode temperature increases linearly when cryostat operating temperature is above 20 mK. Thus, we get the initial thermal phonon occupation  $N_{m^{\text{th}}} = 476$ .

We now present the measured PSD as increasing the sideband cooling power in Supplementary Figure 4b. From top to bottom, the sideband cooling power is increased. From Supplementary Figure 4b we found that the sideband cooling power increases the total mechanical linewidth and the baseline of the measured PSD rises up under strong sideband pump power. The background increasing of measured PSD indicates that the cavity mode is heated and the effective mode temperature can not be viewed as zero-temperature. We add a tunable filter at room temperature with a feedback-loop to maintain the filter frequency matches the device cavity resonance. However, the cavity heating is still there and the cavity heating mainly due to thermal effect caused by defects and poor thermal conductivity of block aluminum superconducting resonators. In the following experiments, the aluminum superconducting material could be replaced by oxygen-free copper to increase the thermal conductivity of microwave resonator. The technical difficulties of cavity field mode heating can also be alleviated by increasing the vacuum coupling strength.
